# Supplementary material for: ACSS-q: Algorithmic complexity for short strings via quantum accelerated approach
Source: arXiv:2009.08866 source file (2020-09-18)
Supplement: Supplementary file 1 [file appendix_1.tex]

% \section{Motivation} \label{sec:motivation}
